# Supplementary material for: Vanishing 2-Qubit Gates with Non-Simplification ZX-Rules
Source: arXiv:2209.06874 source file (2022-09-14)
Supplement: Supplementary file 1 [file appendix1.tex]

\chapter[Proofs]{Proofs} \label{ch:a1}

\kant[1-3]
{\allowdisplaybreaks
\begin{align*}
left &= right1 \\
     &= right2.
\end{align*}}
Here we include the proof for generalized local complementation:
{\allowdisplaybreaks
\begin{align*}
  \tikzfig{gen-lc-proof/0} &= \tikzfig{gen-lc-proof/1} \\
  &= \tikzfig{gen-lc-proof/2} \\
  &= \tikzfig{gen-lc-proof/3} \\
  &= \tikzfig{gen-lc-proof/4} \\
  &= \tikzfig{gen-lc-proof/5}
\end{align*}}
% \ctikzfig{gen-lc-full}
